# Supplementary material for: Boundary Integral Formulation of the Cell-by-Cell Model of Cardiac Electrophysiology
Source: arXiv:2302.05281 source file (2023-02-10)
Supplement: Supplementary file 1 [file CV_all.tex]

\documentclass[crop,tikz,dvipsnames,
class=elsarticle,% underlying class which is loaded by standalone
]{standalone}
\usepackage{currfile}
\usepackage{bm}

\usepackage{\currfile ../../../mycommands}
\usepackage{\currfile ../../../plot_options}

\begin{document}
\begin{tikzpicture}

\pgfplotscreateplotcyclelist{mycolorlisttest}{%
color=colorone,mark=\markone\\
color=colortwo,mark=\marktwo\\
color=colorthree,mark=\markthree\\
color=colorfour,mark=\markfour\\
color=colorfive,mark=\markfive\\
color=colorsix,mark=\marksix\\
}

\pgfplotsset{
    log x ticks with fixed point/.style={
    xticklabel={
      \pgfkeys{/pgf/fpu=true}
      \pgfmathparse{exp(\tick)}%
      \pgfmathprintnumber[fixed relative, precision=3]{\pgfmathresult}
      \pgfkeys{/pgf/fpu=false}
    }
  },
}

\begin{groupplot}[
        group style = {
            group size=2 by 1,
            horizontal sep=1.5cm,
        },
        grid = major,
        width = 7.5cm,
        height = 5.5cm,
        title style = {text width = 6cm},
        cycle list name = mycolorlisttest,
        legend cell align=left,
        legend pos = north west,
        xmode=log,
        title style={anchor=north, yshift=4ex},
        %log x ticks with fixed point,
        every axis plot/.append style=
        {
            solid,
            line width=\plotlinewidth pt,
            mark size=\plotmarksizeu pt,
        },
        tick label style = {font=\footnotesize},
        ylabel = {CV [\si{\meter\per\second}]},
    ]
    
    %%%%%%%%%%%%%%%%%%%
    \nextgroupplot[
        title={\subcaption{CV as function of permeability $\kappa$\label{fig:cv_vs_kappa}}},
        xlabel={$\kappa$ [\si{\milli\siemens\per\square\centi\metre}]},
    ]
    %%%%%%%%%%%%%%%%%%%
    
    \addplot+ table [x=k,y=CV,col sep=comma] {\currfiledir CVl_C_Rl_cl_100.csv};
    \addlegendentry{$c_l=\SI{100}{\um}$}
    \addplot+ table [x=k,y=CV,col sep=comma] {\currfiledir CVl_C_Rl_cl_50.csv};
    \addlegendentry{$c_l=\SI{50}{\um}$}

    %%%%%%%%%%%%%%%%%%%
    \nextgroupplot[
        title={\subcaption{CV as function of conductivity $\sigma_i$\label{fig:cv_vs_si}}},
        extra x ticks = {3},
        extra x tick labels = {3},
        extra x tick style = {color=red,major grid style=red,},
    ]
    %%%%%%%%%%%%%%%%%%%
    
    \addplot+ table [x=si,y=CV,col sep=comma] {\currfiledir CVl_C_si_cl_100.csv};
    \addlegendentry{$c_l=\SI{100}{\um}$}
    \addplot+ table [x=si,y=CV,col sep=comma] {\currfiledir CVl_C_si_cl_50.csv};
    \addlegendentry{$c_l=\SI{50}{\um}$}

\end{groupplot}
\end{tikzpicture}
	
\end{document}
